# Supplementary material for: Dark Matter Benchmark Models for Early LHC Run-2 Searches: Report of the ATLAS/CMS Dark Matter Forum
Source: arXiv:1507.00966 source file (2015-07-03)
Supplement: Supplementary file 1 [file TTBar_Xsecs_Appendix.tex]

\section{\texorpdfstring{Relic density constraints for $b-$flavored Dark Matter}{Relic density constraints for b-flavored Dark Matter}}
\label{app:Relic_Density_bFDM}
\label{app:xsecs_bFDM}

For Dirac fermion DM the relic density is governed primarily by the $s$-wave annihilation cross section, which is given approximately given by:
\begin{equation}
\langle \sigma v \rangle = \frac{3g^4}{32\pi} \frac{m^2_\chi \sqrt{1-(m_b/m_\chi)^2}}{\left( m^2_\Phi+m^2_\chi-m^2_b \right)} \approx \frac{3g^4 m^2_\chi}{32\pi (m^2_\Phi+m^2_\chi)}
\end{equation}

We assume $ \langle \sigma v \rangle=1.5$~pb. 

%For Majorana fermion DM the relic density is governed primarily by the $p$-wave annihilation cross section, which is given approximately by
%\begin{equation}
% \langle \sigma v \rangle \approx a+bv^2,~ b=g^4\frac{m^2_\chi (m^4_B + m^4_\chi)}{16 \pi (m^2_B+m^2_\chi)}
%\end{equation}

Figure~\ref{fig:relic_weights} shows the couplings for various dark matter and mediator massed required to obtain the correct relic density observed in the early universe.

\begin{figure}[h!]
	\centering 
	\includegraphics[scale=0.5]{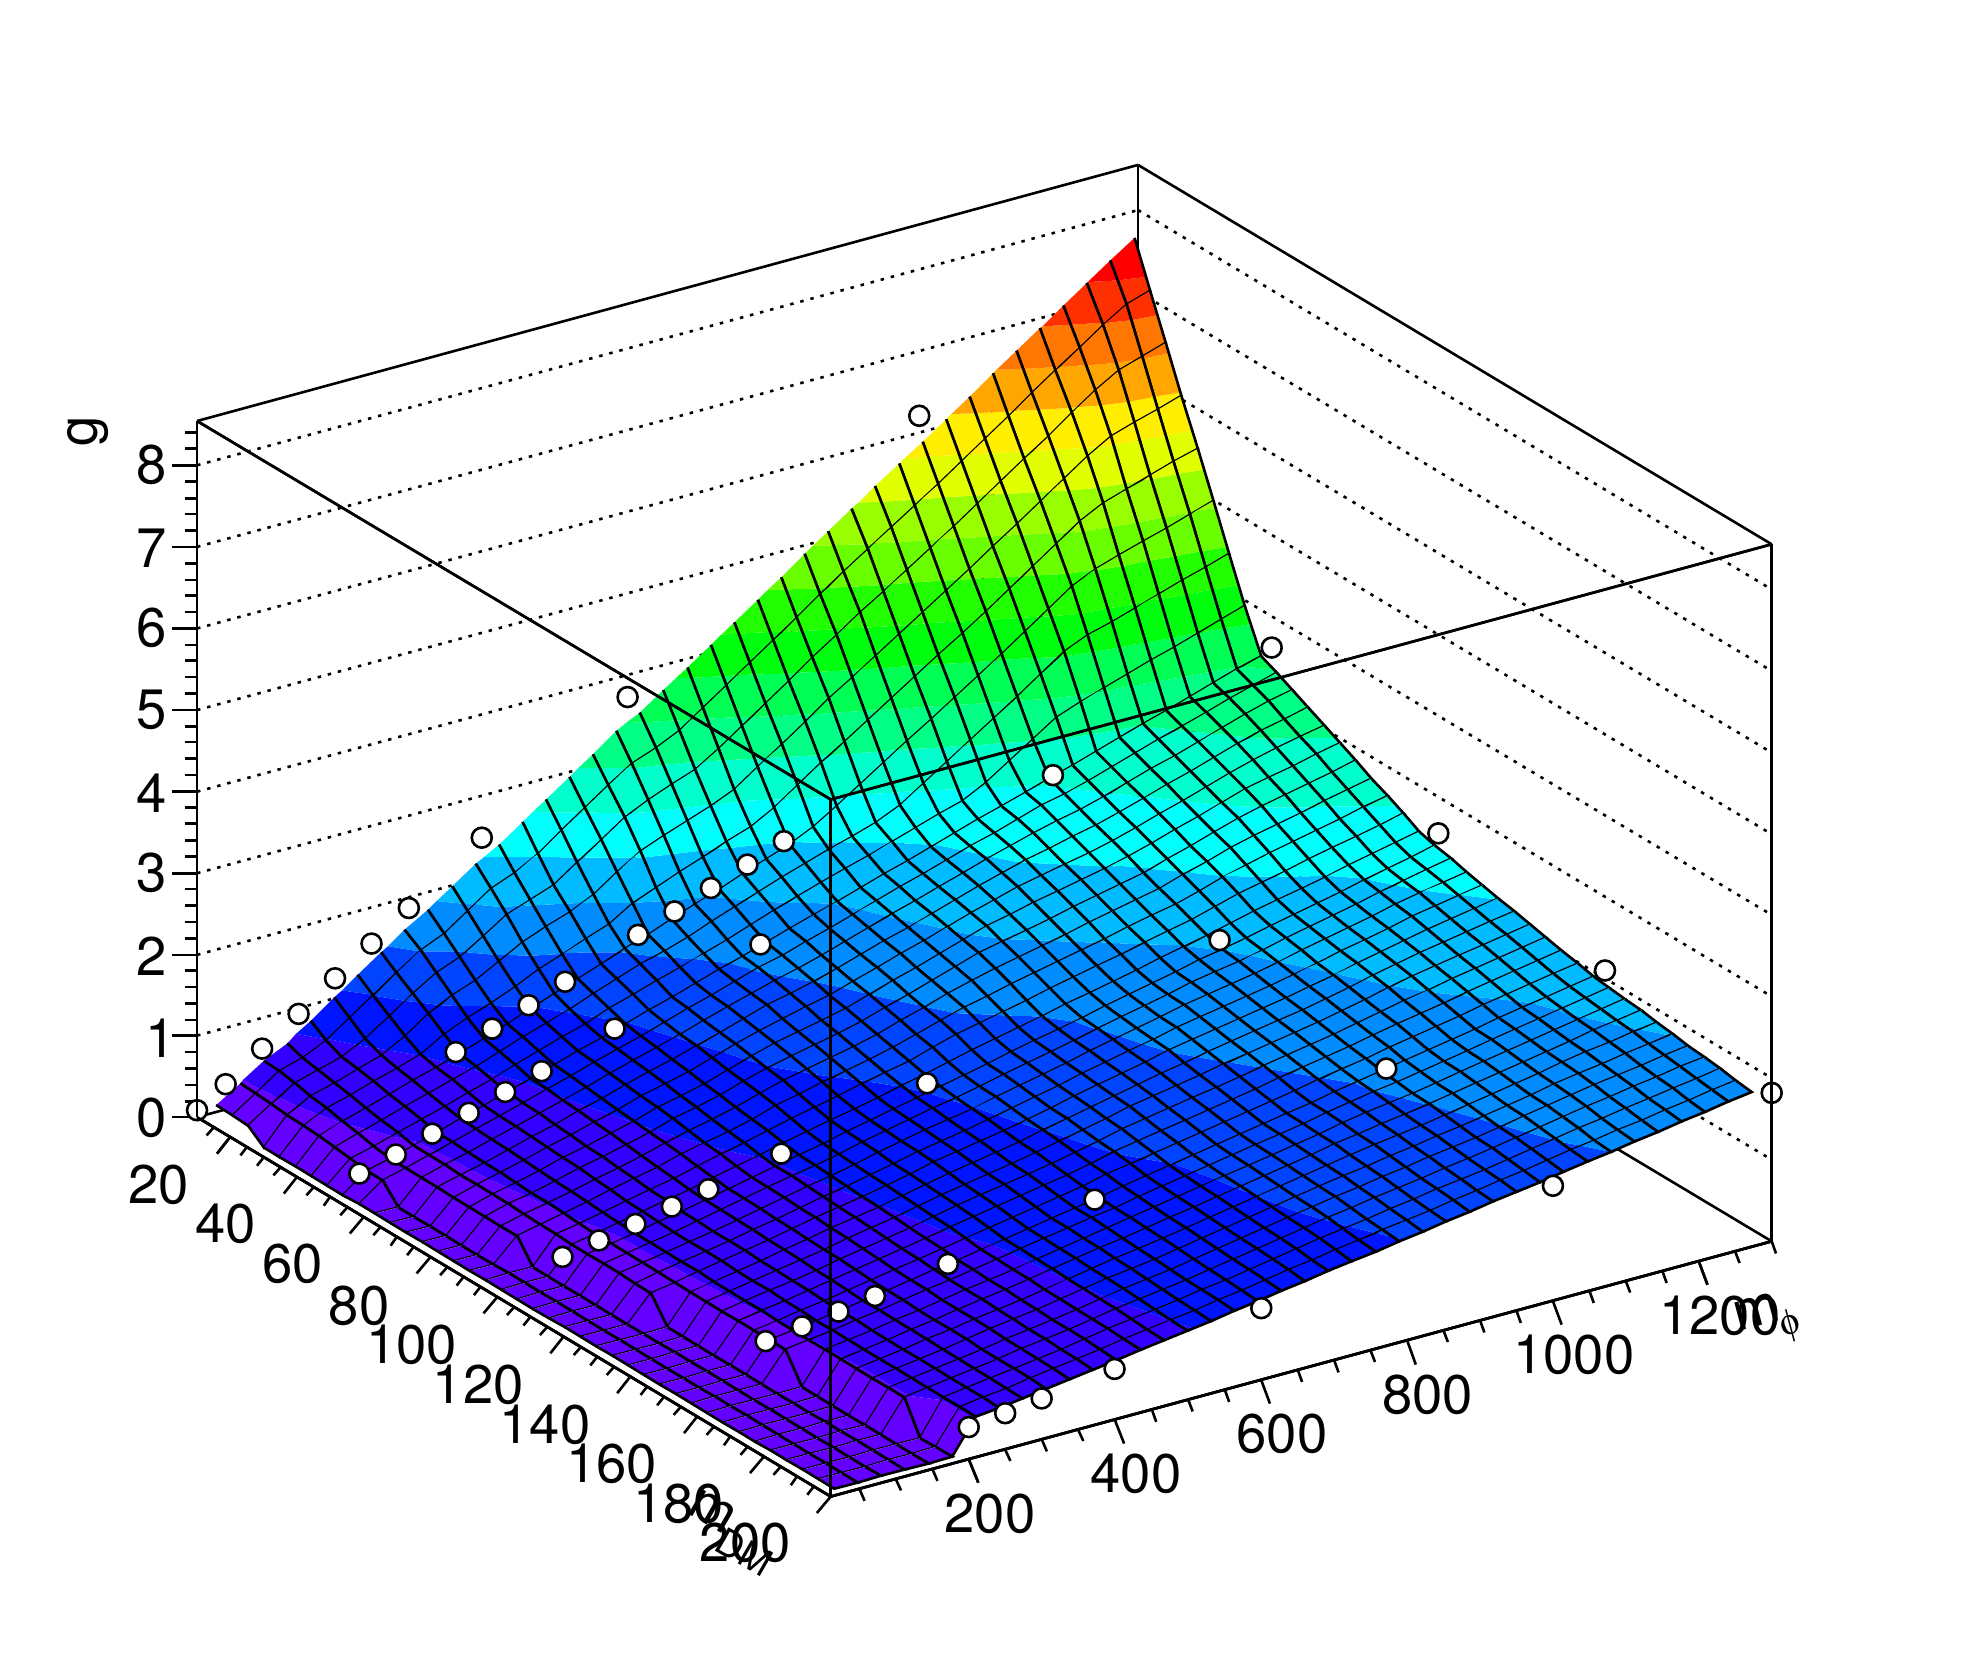}
	\caption{Coupling constants required to obtain correct relic density in the early universe . \label{fig:relic_weights}}
	\end{figure}	

Cross-sections will be made public in a Forum repository TBC.

\section{\texorpdfstring{Cross sections for the $t\bar t$+DM scalar simplified model}{Cross sections for the ttbar+DM scalar simplified model}}

Cross-sections will be made public in a Forum repository TBC. 
