# Supplementary material for: Dark Matter Benchmark Models for Early LHC Run-2 Searches: Report of the ATLAS/CMS Dark Matter Forum
Source: arXiv:1507.00966 source file (2015-07-03)
Supplement: Supplementary file 2 [file appendixCommands.tex]

\makeatletter% since we're using commands with @ in their name
\let\origappendix\appendix% save a copy of the original meaning of \appendix
\renewcommand{\appendix}{%
  \origappendix% do all the original \appendix stuff
  \titlecontents{chapter}%
    [0em] % distance from left margin
    {\vspace{1.5\baselineskip}\begin{fullwidth}\LARGE\rmfamily\itshape} % above (global formatting of entry)
    {\hspace*{0em}\appendixname~\thecontentslabel: } % before w/label (label = ``2'')
    {\hspace*{0em}} % before w/o label
    {\rmfamily\upshape\qquad\thecontentspage} % filler + page (leaders and page num)
    [\end{fullwidth}] % after
  \titleformat{\chapter}%
    [display]% shape
    {\relax\ifthenelse{\NOT\boolean{@tufte@symmetric}}{\begin{fullwidth}}{}}% format applied to label+text
    {\itshape\huge Appendix~\thechapter}% label
    {0pt}% horizontal separation between label and title body
    {\huge\rmfamily\itshape}% before the title body
    [\ifthenelse{\NOT\boolean{@tufte@symmetric}}{\end{fullwidth}}{}]% after the title body
  \setcounter{tocdepth}{1}
  \setcounter{secnumdepth}{1}
  %
  % Add any other special appendix-related code here.
  %
}
\makeatother% restore the special meaning of @
%restore the title
